# Supplementary material for: Ab initio Investigation of Structural Stability and Exfoliation Energies in Transition Metal Dichalcogenides based on Ti-, V-, and Mo-Group Elements
Source: arXiv:1903.08112 ancillary file (2019-03-19)
Supplement: Supplementary file 1 [file supplemental_materials_TMDs.pdf]

# Supplementary Materials: Ab-initio Investigation of Structural Stability and Exfoliation Energies in Transition Metal Dichalcogenides based on Ti-, V-, and Mo-Group Elements

Carlos M. O. Bastos,[1] Rafael Besse,[1] Juarez L. F. Da Silva,[2] and Guilherme M. Sipahi[1]

[1]*São Carlos Institute of Physics, University of São Paulo, PO Box 369, 13560-970, São Carlos, SP, Brazil.*
[2]*São Carlos Institute of Chemistry, University of São Paulo, PO Box 780, 13560-970, São Carlos, SP, Brazil.*

## I. COMPUTATIONAL DETAILS

TABLE I. PAW VASP projectors used in this work, with the number of valence electrons (ZVAL) and the cut-off energies recommended by VASP, used in the minimization of the stress/elastic constants tensor and in the determination of the total energy/band structures.

| | | | | cut-off energy (eV) | |
|---|---|---|---|---|---|
| specie | PAW | valence | recommended | stress/elastic | total energy/band structure |
| S | PAW_PBE S 06Sep2000 | 6 | 258.689 | 517.378 | 291.025 |
| Se | PAW_PBE Se 06Sep2000 | 6 | 211.555 | 423.110 | 237.999 |
| Te | PAW_PBE Te 08Apr2002 | 6 | 174.982 | 349.964 | 196.854 |
| Ti | PAW_PBE Ti 08Apr2002 | 5 | 178.330 | 356.660 | 200.621 |
| Zr | PAW_PBE Zr_sv 04Jan2005 | 12 | 229.898 | 459.796 | 258.635 |
| Hf | PAW_PBE Hf 20Jan2003 | 4 | 220.334 | 440.668 | 247.875 |
| V | PAW_PBE V 08Apr2002 | 5 | 192.543 | 385.086 | 216.610 |
| Nb | PAW_PBE Nb_pv 08Apr2002 | 11 | 208.608 | 417.216 | 234.684 |
| Ta | PAW_PBE Ta 17Jan2003 | 5 | 223.667 | 447.334 | 251.625 |
| Cr | PAW_PBE Cr 06Sep2000 | 6 | 227.080 | 454.160 | 255.465 |
| Mo | PAW_PBE Mo 08Apr2002 | 6 | 224.584 | 449.168 | 252.657 |
| W | PAW_PBE W 08Apr2002 | 5 | 223.057 | 446.114 | 250.939 |

# II. CONVERGENCE TESTS

## A. k-points density

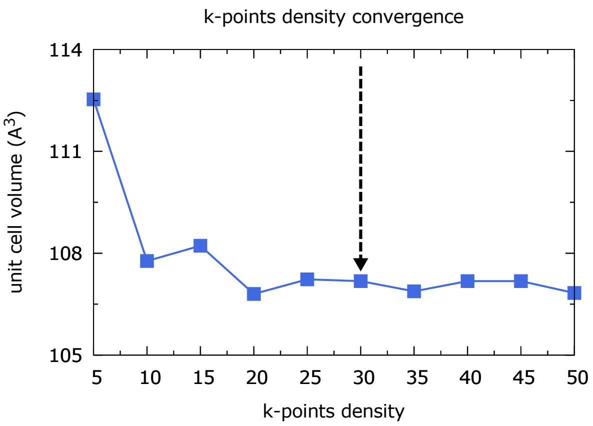


FIG. 1. Convergence test using $MoS_2$ in 2H phase, showing the dependence of volume unit cell with k-point density (in left) and cutoff energy (right).

## B. Cut-off energy

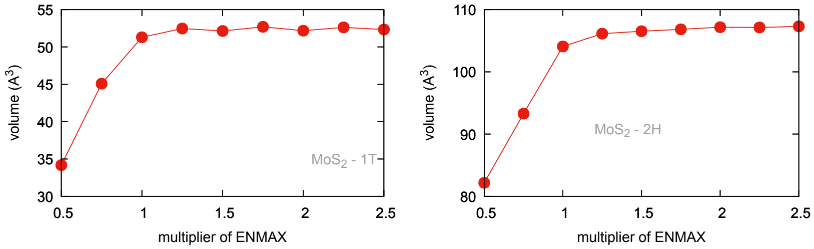


FIG. 2. Convergence test for cut-off energy using $MoS_2$ in 1T (left) and 2H (right) phase.

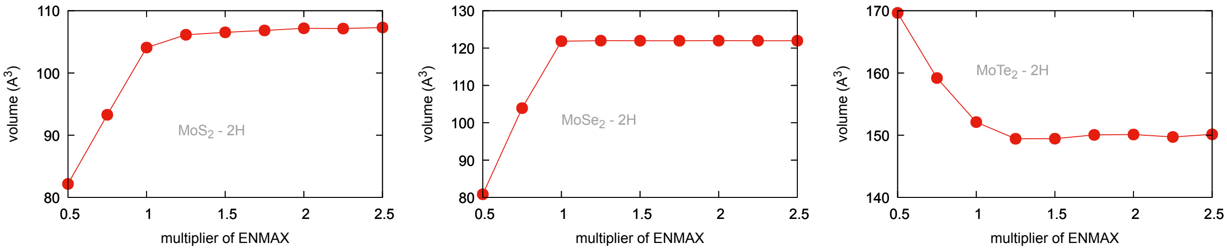


FIG. 3. Convergence test for cut-off energy for $MoS_2$, $MoSe_2$ and $MoTe_2$ in 2H phase.

## III. INITIAL MAGNETIC CONFIGURATIONS

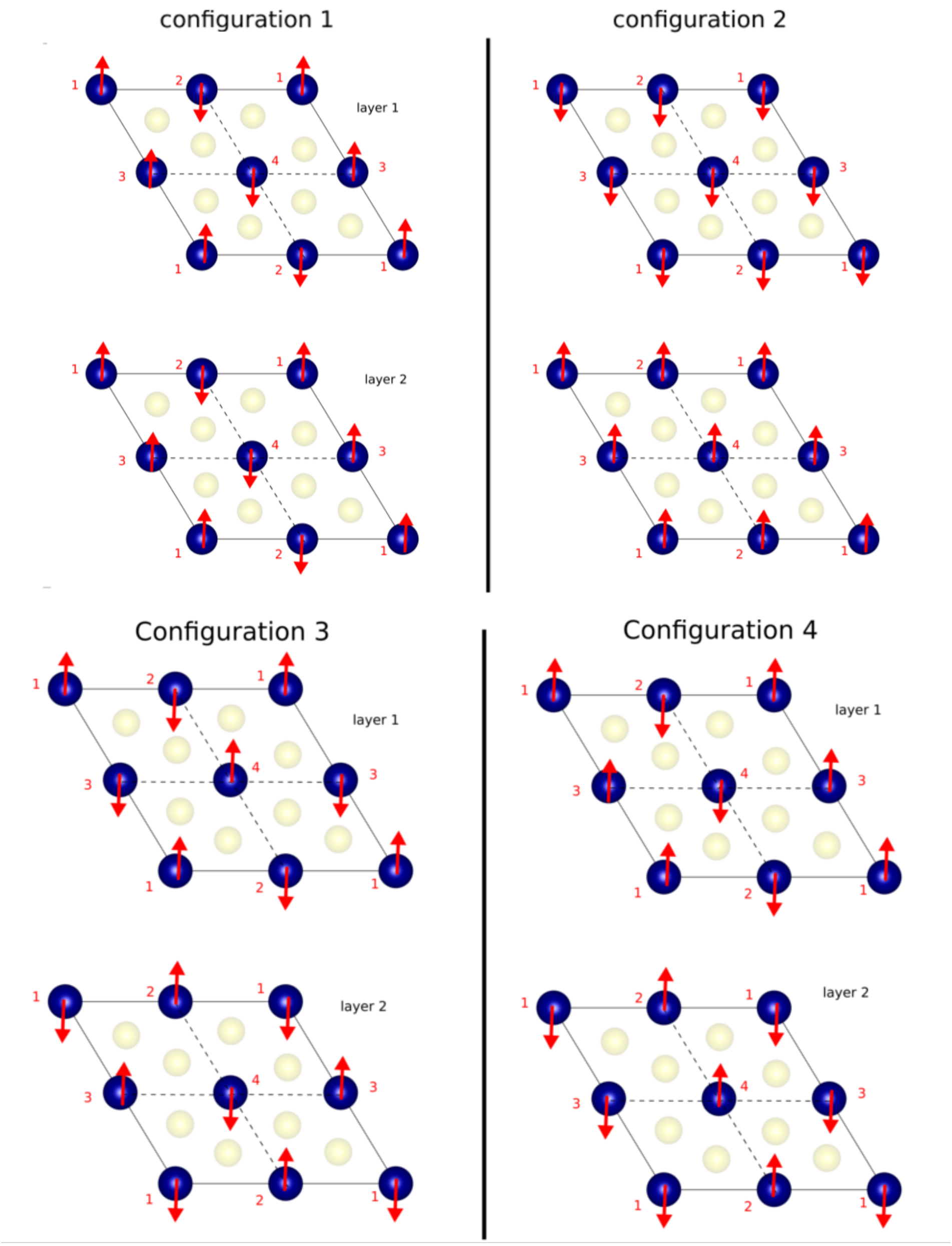


FIG. 4. Initial magnetic configurations. Arrows represent the magnetic moment in the metal element.

## IV. RELATIVE ENERGY

TABLE II. Relativity energy between 1T and $1T_d$ in comparison with 2H phase, by atom. All energies are in meV

| | energy (1T-2H) | energy ($1T_d$-2H) |
|---|---|---|
| $TiS_2$ | −144 | - |
| $TiSe_2$ | −125 | - |
| $TiTe_2$ | −112 | - |
| $ZrS_2$ | −191 | - |
| $ZrSe_2$ | −151 | - |
| $ZrTe_2$ | −115 | - |
| $HfS_2$ | −217 | - |
| $HfSe_2$ | −179 | - |
| $HfTe_2$ | −139 | - |
| $VS_2$ | 12 | - |
| $VSe_2$ | 8 | - |
| $VTe_2$ | −4 | −24.1 |
| $NbS_2$ | 22 | - |
| $NbSe_2$ | 17 | - |
| $NbTe_2$ | 6 | −8 |
| $TaS_2$ | 13 | - |
| $TaSe_2$ | 13 | - |
| $TaTe_2$ | −2 | −36 |
| $CrS_2$ | 176 | 107 |
| $CrSe_2$ | −32 | 53 |
| $CrTe_2$ | −103 | - |
| $MoS_2$ | 271 | 183 |
| $MoSe_2$ | 227 | 112 |
| $MoTe_2$ | 170 | 18 |
| $WS_2$ | 292 | 178 |
| $WSe_2$ | 252 | 96 |
| $WTe_2$ | 188 | −21 |

## V. ELASTIC CONSTANTS

TABLE III. TMDs bulk materials elastic constants for phases 1T, 2H and $1T_d$. Only the non-zero values are given according to the respective crystal symmetry. Some materials are unstable when in $1T_d$ phase. All values are given in GPa.

| | 1T | | | | | | | 2H | | | | | | $1T_d$ | | | | | | | | |
|---|---|---|---|---|---|---|---|---|---|---|---|---|---|---|---|---|---|---|---|---|---|---|
| | $C_{11}$ | $C_{12}$ | $C_{13}$ | $C_{14}$ | $C_{33}$ | $C_{44}$ | $C_{66}$ | $C_{11}$ | $C_{12}$ | $C_{13}$ | $C_{33}$ | $C_{44}$ | $C_{66}$ | $C_{11}$ | $C_{12}$ | $C_{13}$ | $C_{22}$ | $C_{23}$ | $C_{33}$ | $C_{44}$ | $C_{55}$ | $C_{66}$ |
| $TiS_2$ | 141 | 32 | 10 | −3 | 30 | 12 | 55 | 140 | 56 | 13 | 40 | 5 | 42 | | | | | unstable | | | | |
| $TiSe_2$ | 103 | 23 | 10 | −3 | 36 | 13 | 40 | 115 | 41 | 15 | 20 | 4 | 37 | | | | | unstable | | | | |
| $TiTe_2$ | 81 | 20 | 15 | −7 | 39 | 19 | 31 | 76 | 25 | 19 | 30 | 1 | 25 | | | | | unstable | | | | |
| $ZrS_2$ | 134 | 26 | 8 | −3 | 34 | 9 | 54 | 138 | 52 | 10 | 30 | 4 | 43 | | | | | unstable | | | | |
| $ZrSe_2$ | 108 | 22 | 7 | −3 | 32 | 10 | 43 | 109 | 43 | 11 | 32 | 4 | 33 | | | | | unstable | | | | |
| $ZrTe_2$ | 69 | 13 | 10 | −5 | 35 | 16 | 28 | 71 | 24 | 14 | 27 | 2 | 23 | | | | | unstable | | | | |
| $HfS_2$ | 148 | 29 | 8 | −3 | 35 | 10 | 60 | 155 | 58 | 9 | 38 | 6 | 49 | | | | | unstable | | | | |
| $HfSe_2$ | 119 | 24 | 7 | −3 | 33 | 10 | 48 | 125 | 45 | 10 | 35 | 6 | 40 | | | | | unstable | | | | |
| $HfTe_2$ | 72 | 13 | 6 | −5 | 28 | 13 | 30 | 80 | 29 | 13 | 32 | 4 | 26 | | | | | unstable | | | | |
| $VS_2$ | 171 | 35 | 11 | −3 | 33 | 12 | 68 | 164 | 57 | 4 | 25 | 9 | 54 | | | | | unstable | | | | |
| $VSe_2$ | 124 | 22 | 18 | −5 | 34 | 11 | 51 | 129 | 42 | 7 | 12 | 8 | 43 | | | | | unstable | | | | |
| $VTe_2$ | 79 | 28 | 22 | −1 | 38 | 21 | 28 | 91 | 31 | 16 | 69 | 13 | 30 | 131 | 31 | 9 | 101 | 34 | 66 | 6 | 24 | 45 |
| $NbS_2$ | 158 | 37 | 9 | −11 | 36 | 13 | 61 | 171 | 56 | 13 | 51 | 5 | 58 | | | | | unstable | | | | |
| $NbSe_2$ | 120 | 33 | 1 | −6 | 26 | 20 | 44 | 140 | 46 | 8 | 46 | 6 | 47 | | | | | unstable | | | | |
| $NbTe_2$ | 101 | 24 | 10 | −11 | 17 | 18 | 39 | 97 | 34 | 6 | 44 | 8 | 31 | 134 | 24 | 16 | 85 | 30 | 74 | 6 | 28 | 45 |
| $TaS_2$ | 178 | 30 | 11 | −5 | 39 | 10 | 74 | 200 | 67 | 7 | 55 | 7 | 67 | | | | | unstable | | | | |
| $TaSe_2$ | 123 | 13 | 4 | −4 | 44 | 14 | 55 | 151 | 54 | 7 | 51 | 8 | 48 | | | | | unstable | | | | |
| $TaTe_2$ | 107 | 23 | 13 | −3 | 28 | 15 | 42 | 100 | 39 | 9 | 44 | 6 | 31 | 152 | 30 | 15 | 115 | 27 | 73 | 6 | 30 | 51 |
| $CrS_2$ | 154 | 7 | 24 | −6 | 41 | 11 | 71 | 204 | 53 | 11 | 47 | 12 | 56 | 206 | 43 | 28 | 189 | 26 | 42 | 5 | 33 | 87 |
| $CrSe_2$ | 103 | 95 | 27 | −1 | 97 | 1 | 39 | 159 | 46 | 10 | 42 | 11 | 39 | 164 | 40 | 29 | 148 | 29 | 34 | 2 | 26 | 64 |
| $CrTe_2$ | 80 | 37 | 24 | −5 | 58 | 18 | 22 | 108 | 100 | 30 | 120 | 15 | 40 | | | | | unstable | | | | |
| $MoS_2$ | 197 | 1 | 27 | −11 | 39 | 19 | 99 | 225 | 54 | 10 | 48 | 15 | 84 | 207 | 34 | 25 | 186 | 26 | 34 | 7 | 22 | 67 |
| $MoSe_2$ | 168 | 9 | 25 | −4 | 40 | 11 | 80 | 177 | 39 | 10 | 44 | 15 | 68 | 182 | 42 | 23 | 160 | 20 | 29 | 3 | 25 | 58 |
| $MoTe_2$ | 131 | 5 | 18 | −3 | 35 | 4 | 63 | 123 | 28 | 9 | 37 | 18 | 47 | 126 | 51 | 25 | 110 | 24 | 27 | 4 | 30 | 49 |
| $WS_2$ | 198 | 1 | 22 | −7 | 40 | 13 | 98 | 240 | 50 | 10 | 52 | 16 | 94 | 231 | 36 | 19 | 197 | 28 | 31 | 5 | 19 | 72 |
| $WSe_2$ | 168 | 5 | 27 | −2 | 37 | 8 | 81 | 195 | 35 | 10 | 48 | 17 | 80 | 206 | 43 | 18 | 177 | 19 | 34 | 3 | 23 | 64 |
| $WTe_2$ | 136 | −3 | 21 | −4 | 34 | 6 | 70 | 135 | 21 | 9 | 40 | 21 | 57 | 170 | 41 | 18 | 96 | 24 | 27 | 1 | 24 | 52 |

## VI. EXFOLIATION ENERGY

TABLE IV. Exfoliation energy.

| | energy (meV/Å$^2$) | | | | energy (meV/Å$^2$) | | | | energy (meV/Å$^2$) | | |
|---|---|---|---|---|---|---|---|---|---|---|---|
| | 1T | 2H | 1T$_d$ | | 1T | 2H | 1T$_d$ | | 1T | 2H | 1T$_d$ |
| $TiS_2$ | 13 | 11 | - | $TiSe_2$ | 14 | 12 | - | $TiTe_2$ | 14 | 13 | - |
| $ZrS_2$ | 10 | 10 | - | $ZrSe_2$ | 11 | 10 | - | $ZrTe_2$ | 13 | 11 | - |
| $HfS_2$ | 10 | 10 | - | $HfSe_2$ | 11 | 11 | - | $HfTe_2$ | 13 | 12 | - |
| $VS_2$ | 15 | 13 | - | $VSe_2$ | 15 | 13 | - | $VTe_2$ | 16 | 15 | 22 |
| $NbS_2$ | 15 | 14 | - | $NbSe_2$ | 17 | 14 | - | $NbTe_2$ | 17 | 16 | 20 |
| $TaS_2$ | 15 | 14 | - | $TaSe_2$ | 16 | 15 | - | $TaTe_2$ | 17 | 16 | 21 |
| $CrS_2$ | 13 | 13 | 16 | $CrSe_2$ | 20 | 13 | 15 | $CrTe_2$ | 20 | 15 | - |
| $MoS_2$ | 15 | 14 | 14 | $MoSe_2$ | 16 | 15 | 14 | $MoTe_2$ | 14 | 15 | 15 |
| $WS_2$ | 15 | 14 | 14 | $WSe_2$ | 16 | 16 | 15 | $WTe_2$ | 15 | 16 | 15 |

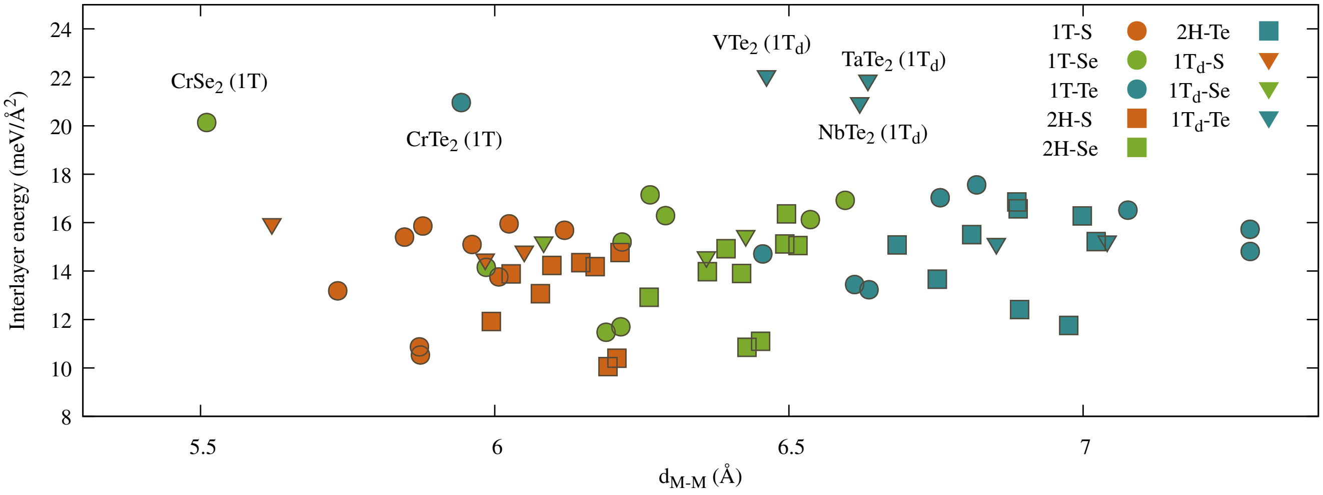


FIG. 5. Exfoliation energy. x-axis is the distance between metals in different layers

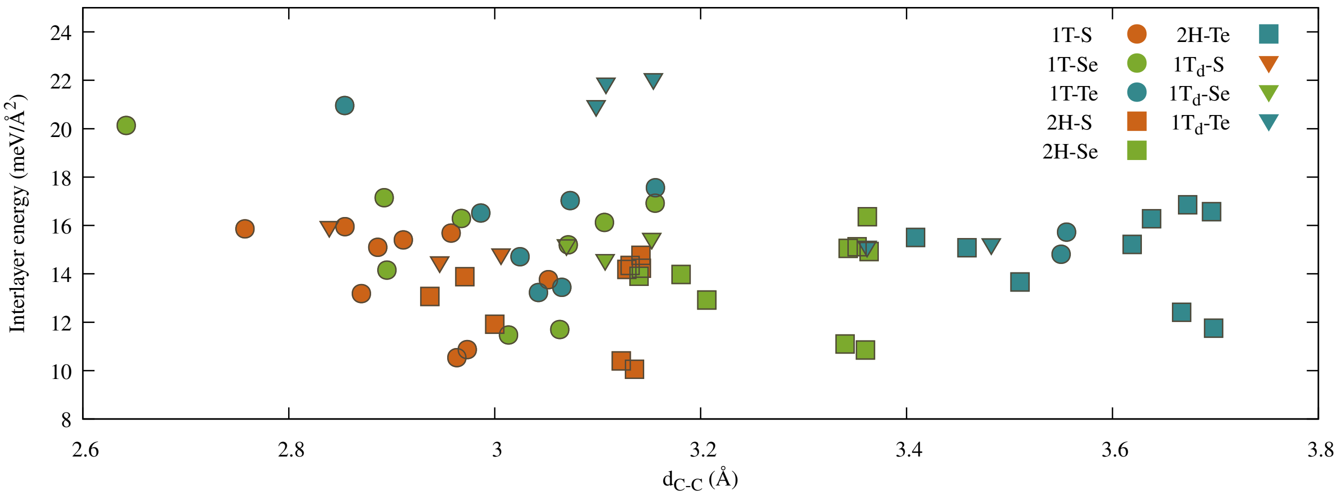


FIG. 6. Exfoliation energy. x-axis is the distance between chalcogen atoms in different layers

## VII. BAND STRUCTURE AND DENSITY OF STATE FOR 2H PHASE

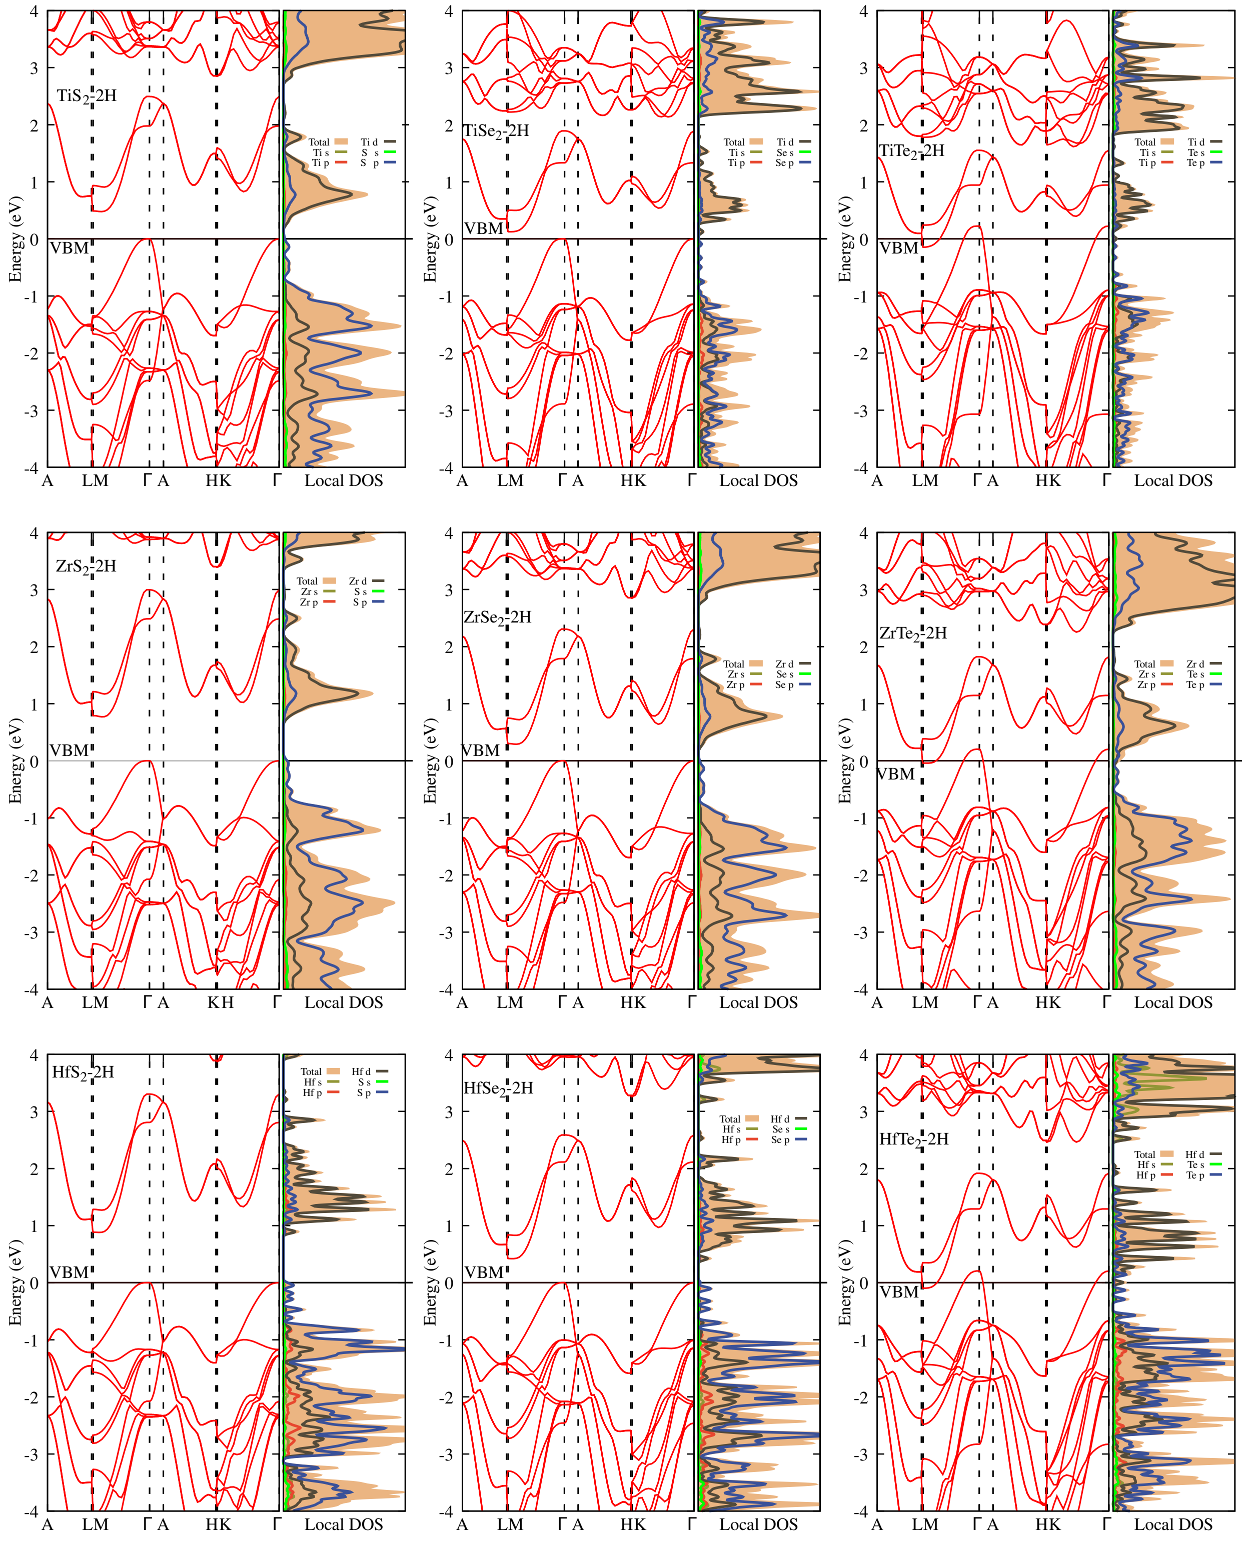


FIG. 7. 2H phase: Ti, Zr, Hf.

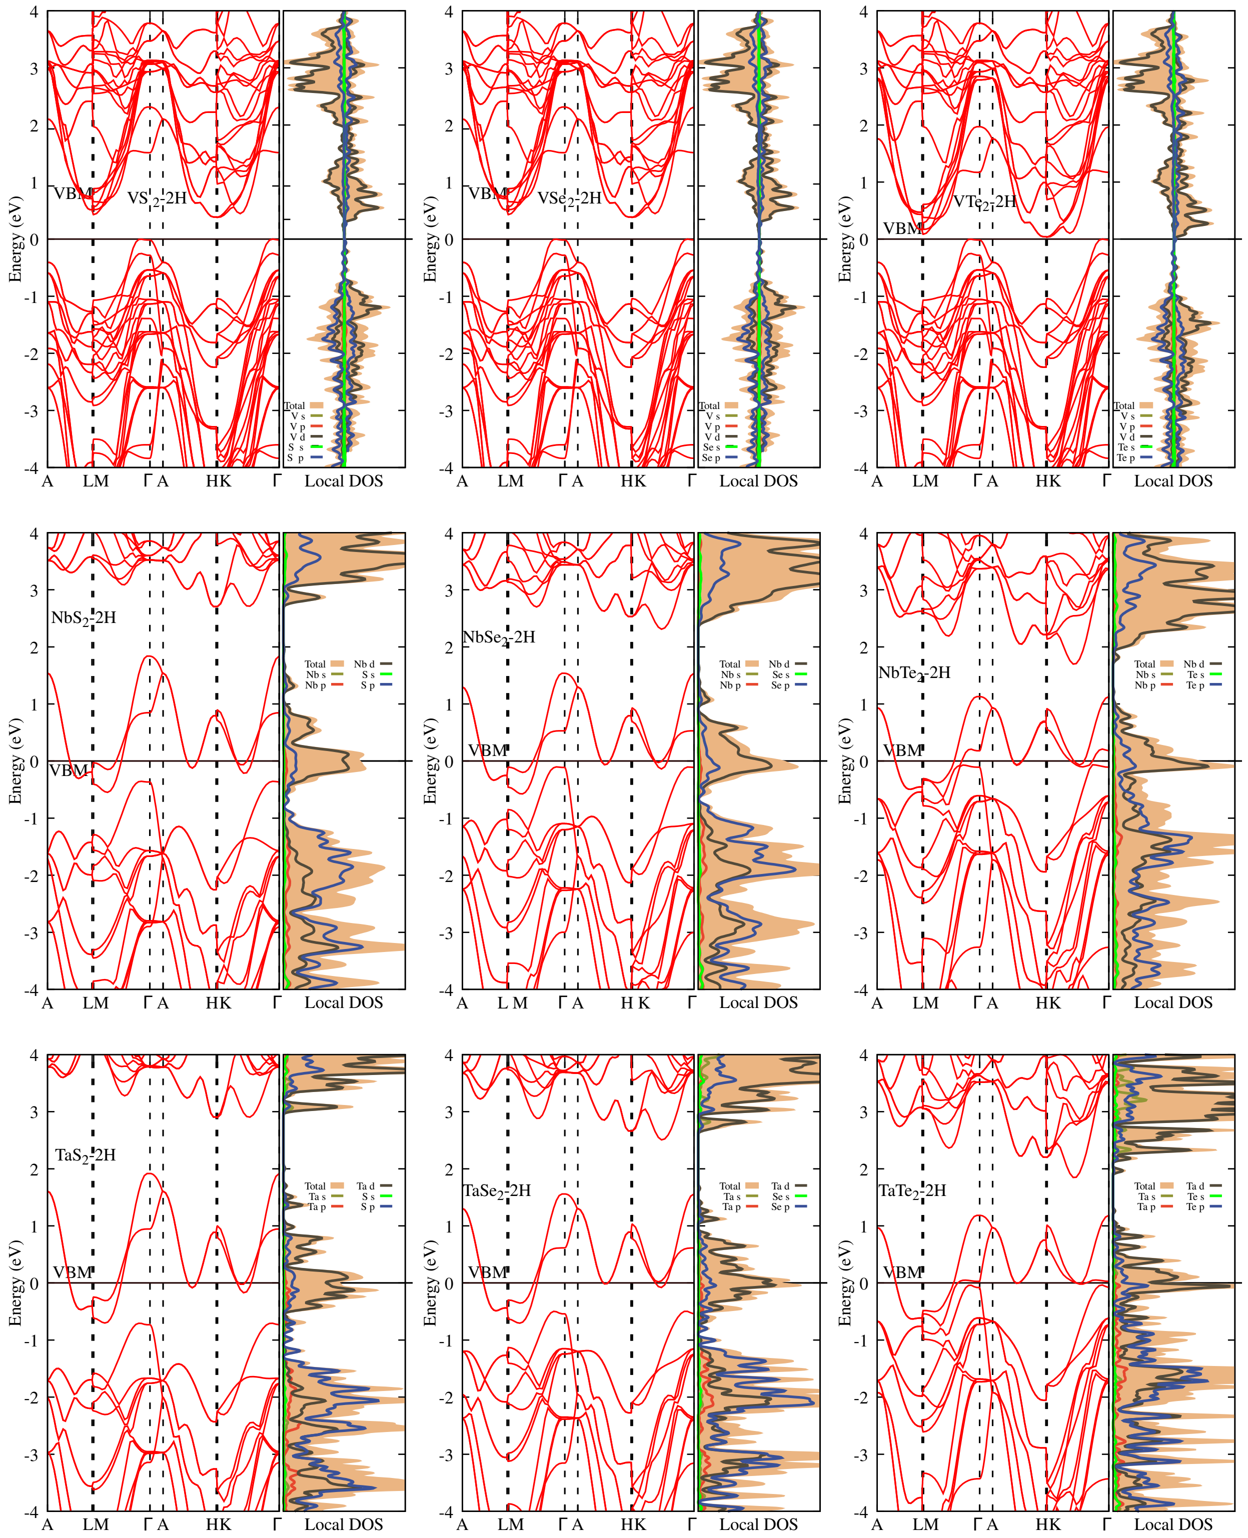


FIG. 8. 2H phase: V, Nb, Ta.

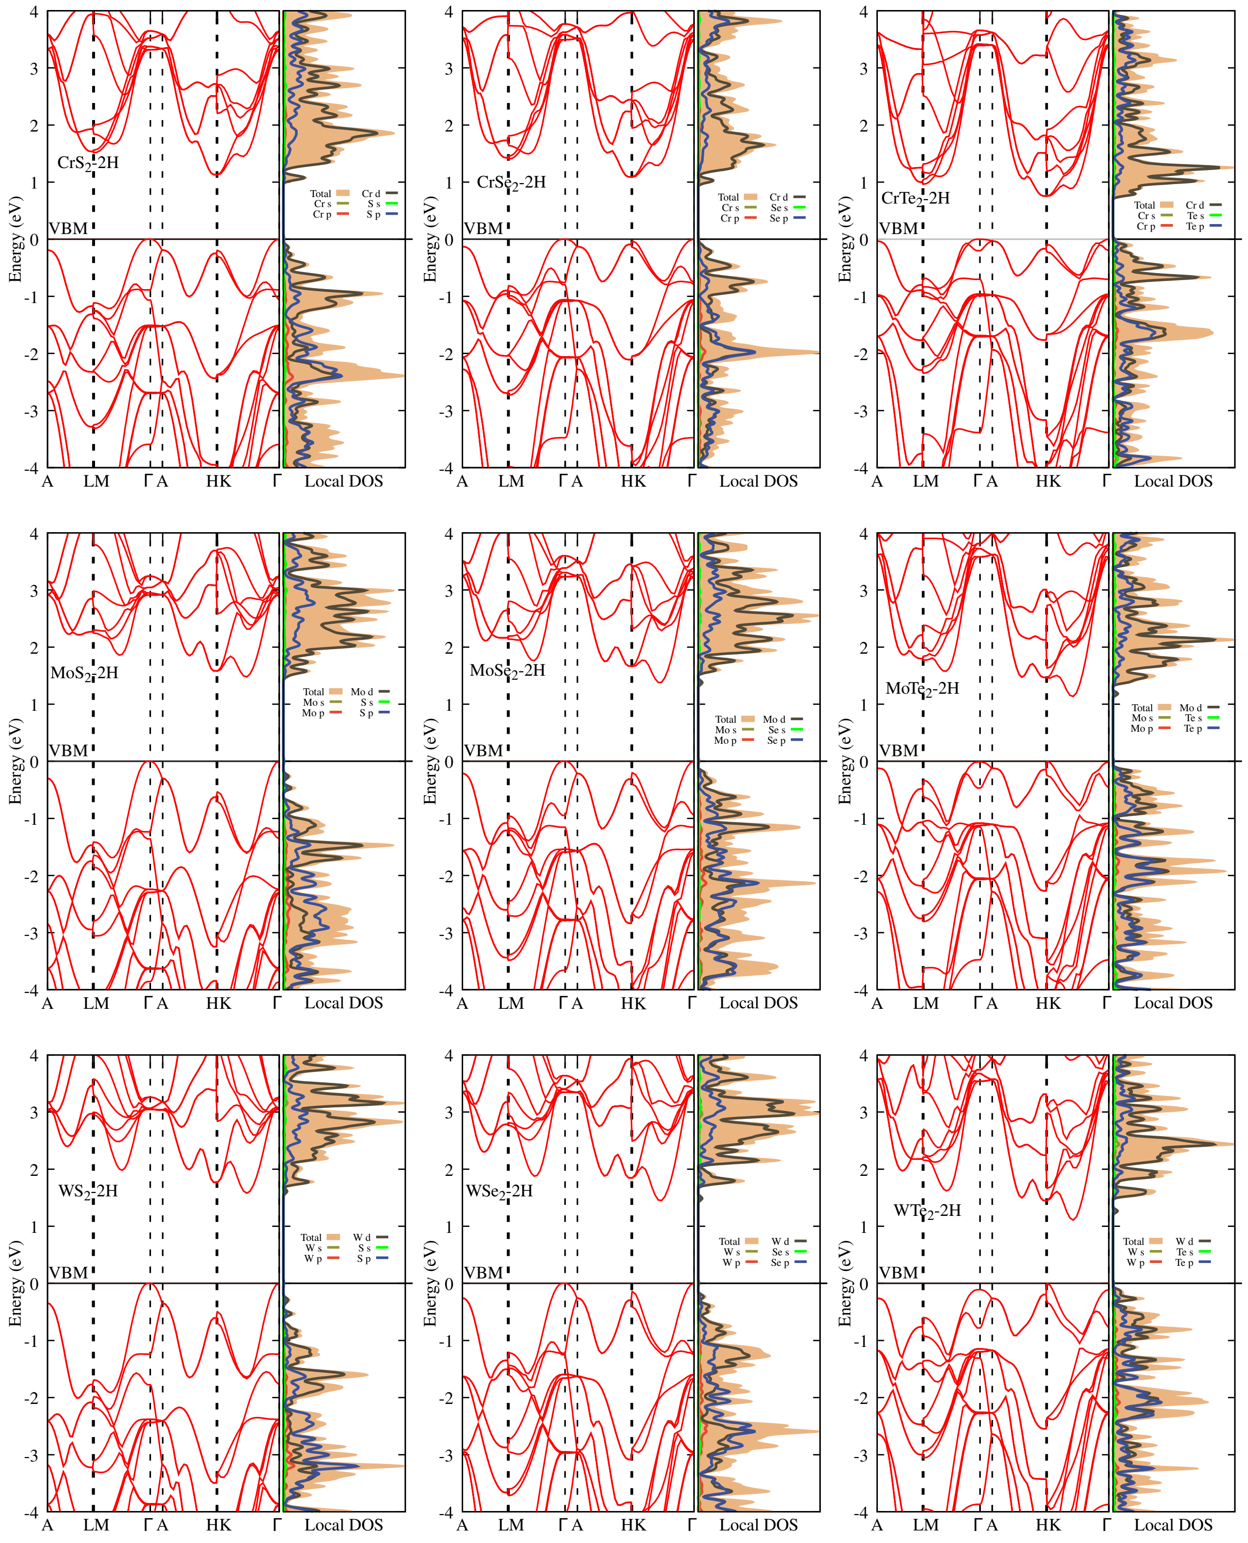


FIG. 9. 2H phase: Cr, Mo, W.

# VIII. BAND STRUCTURE AND DENSITY OF STATE FOR 1T PHASE

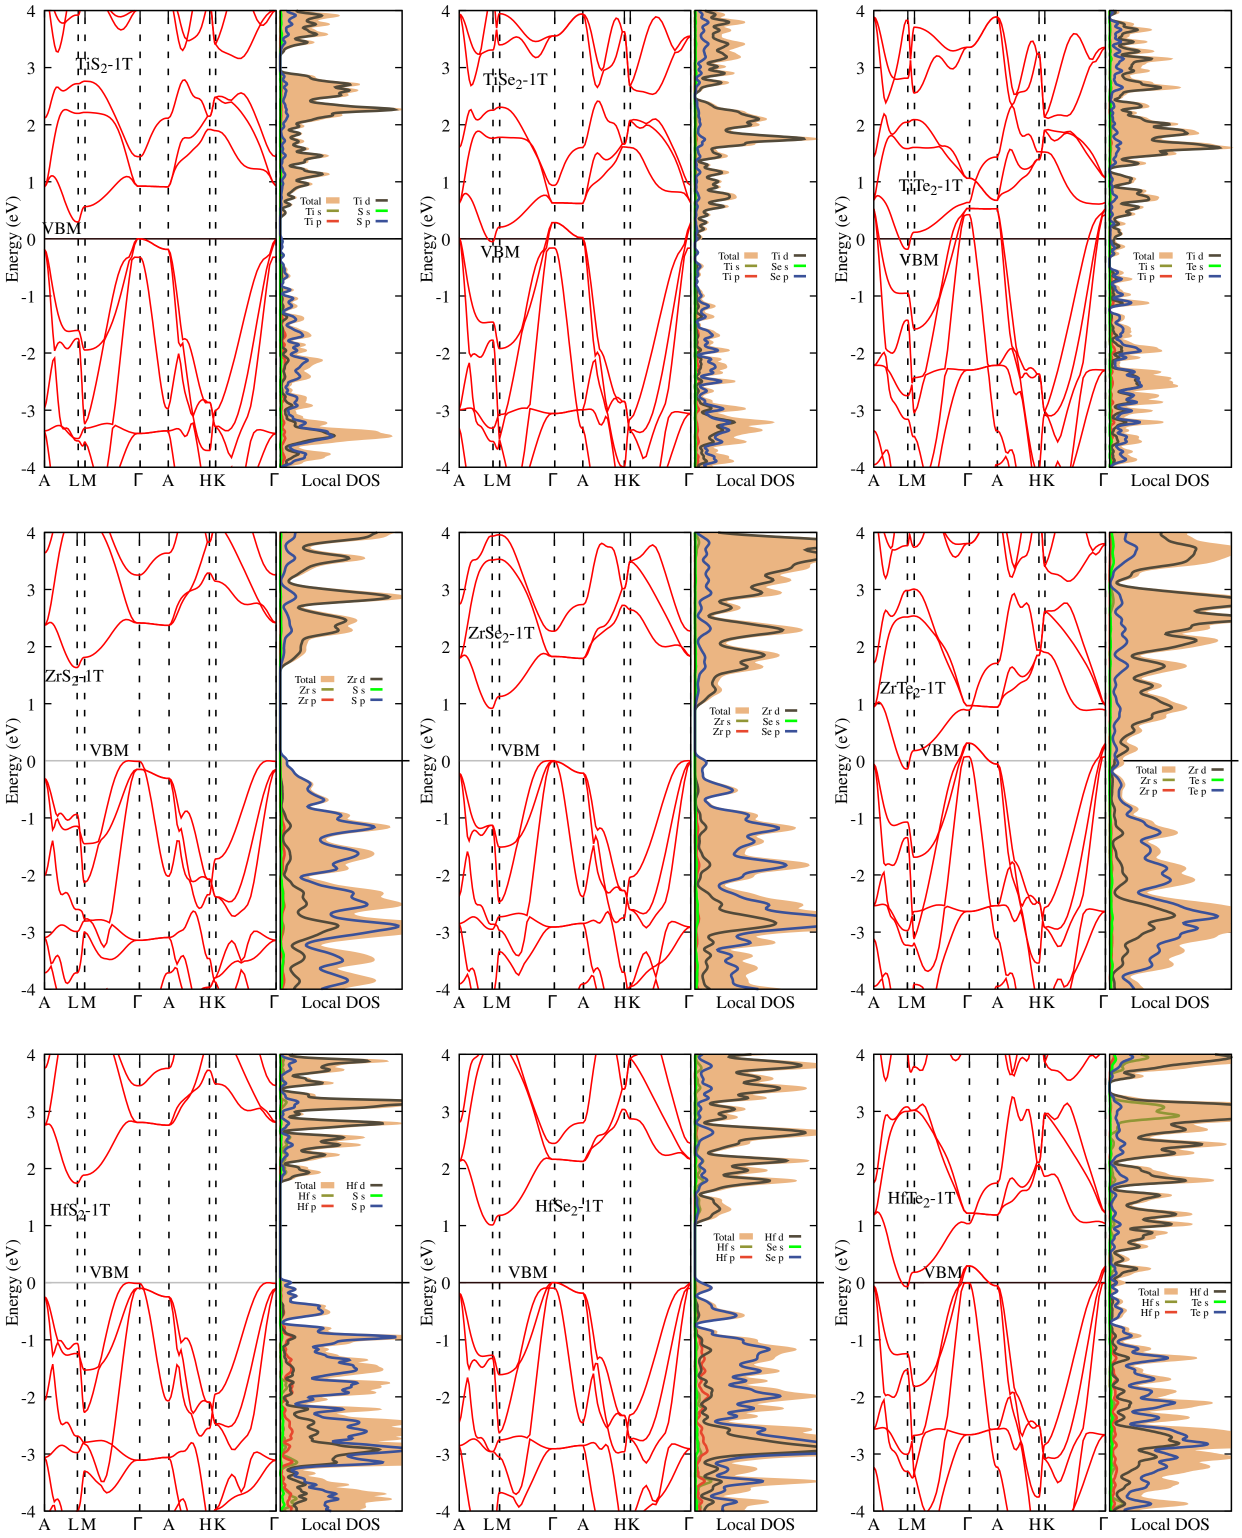

FIG. 10. 1T: Ti, Zr, Hf

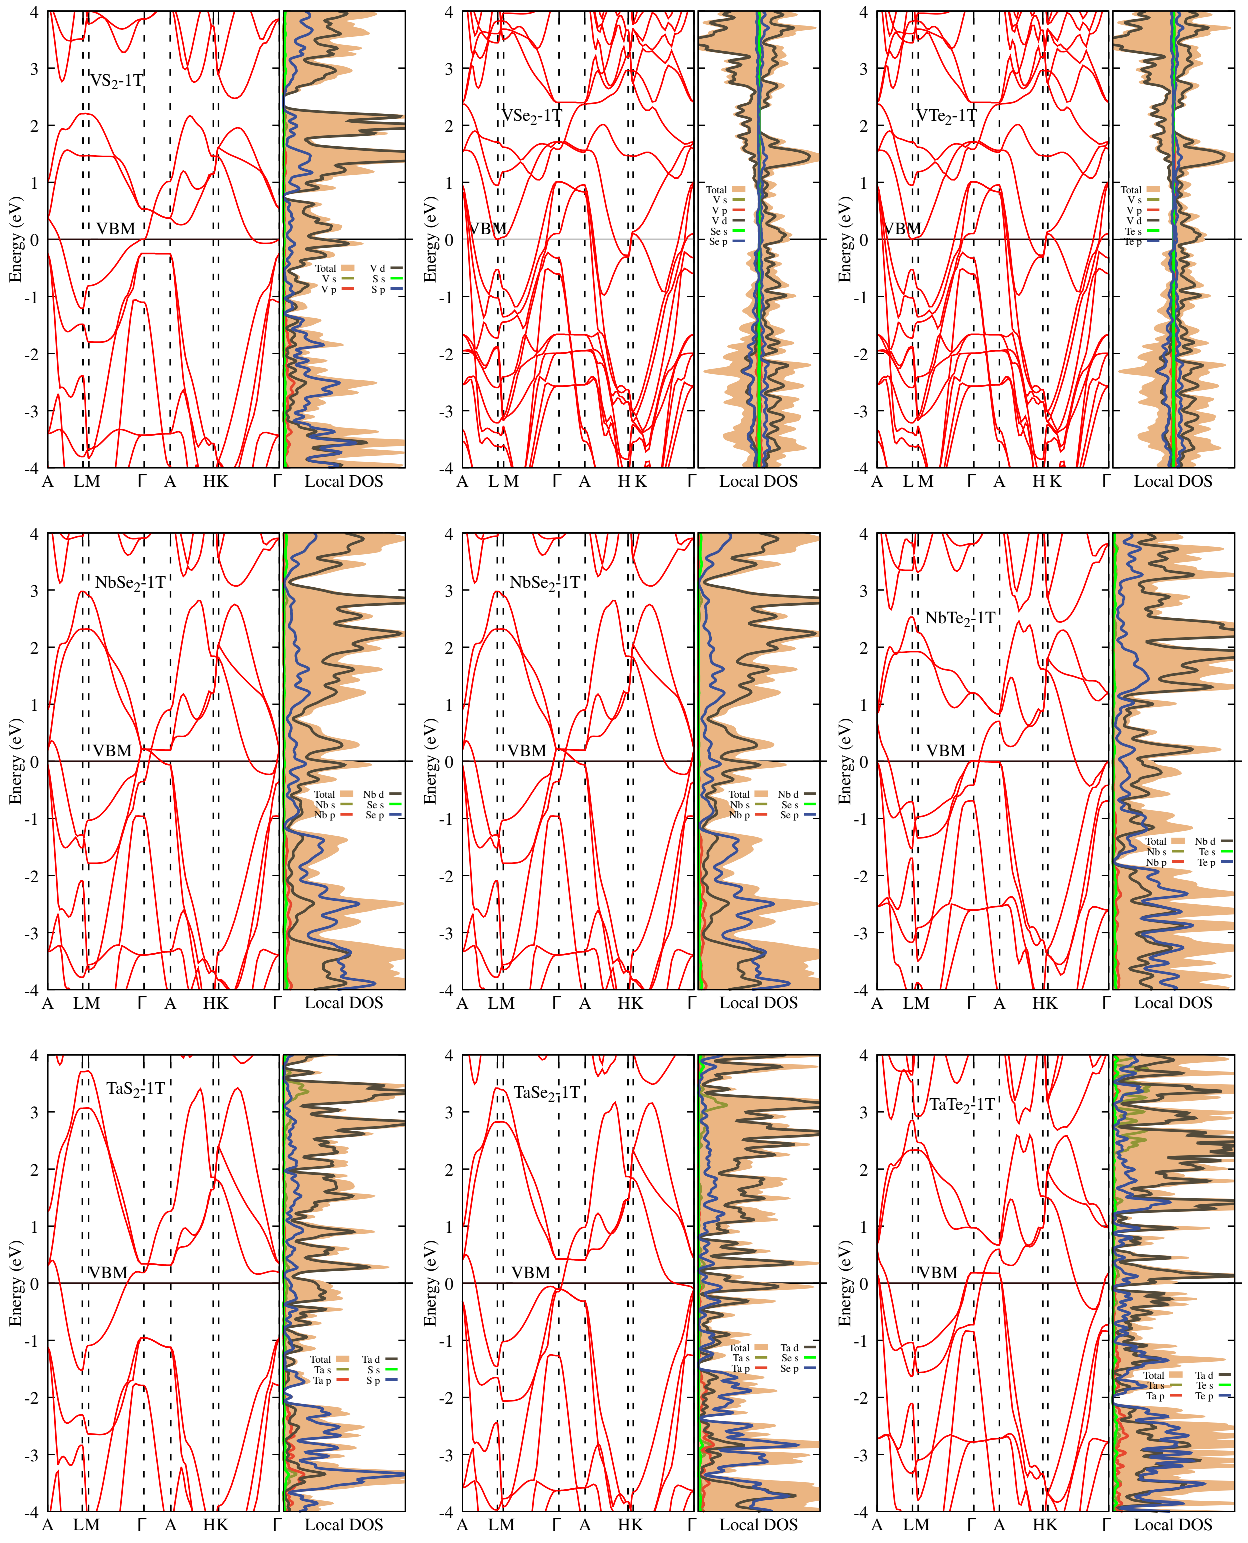


FIG. 11. 1T phase: V, Nb, Ta.

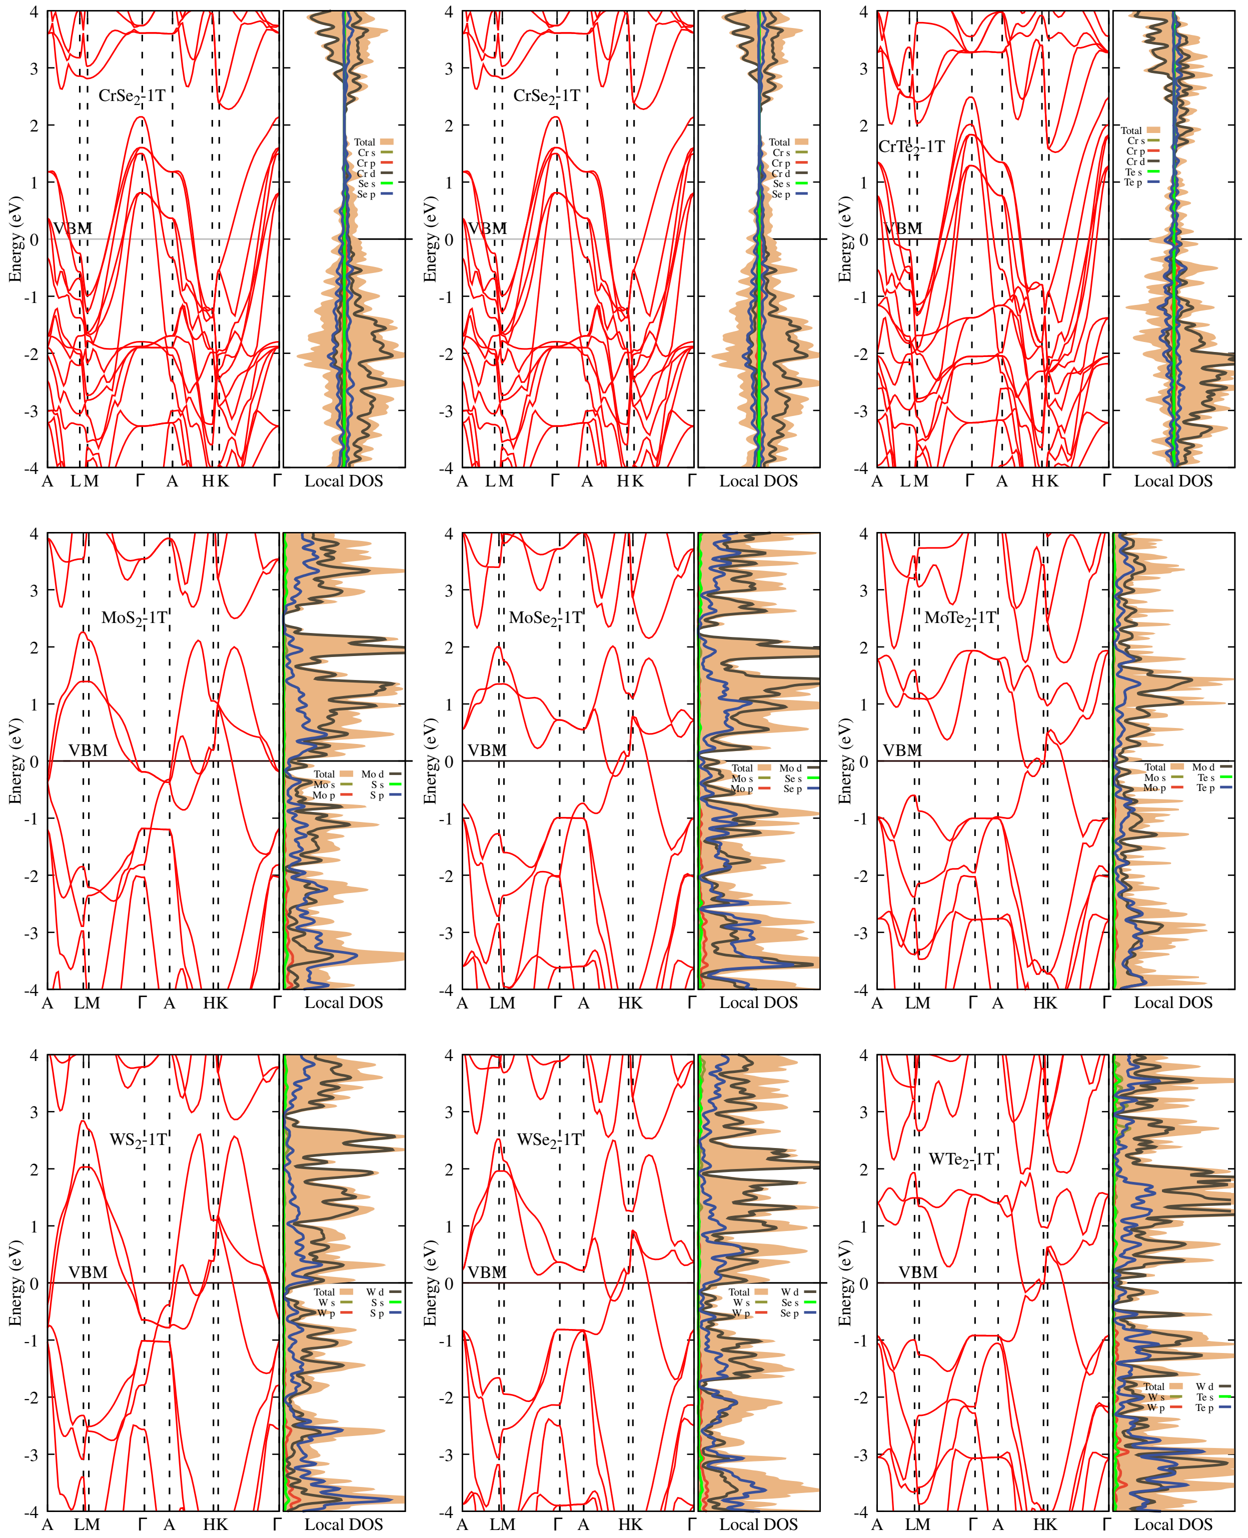


FIG. 12. 1T: Cr, Mo, W

## IX. BAND STRUCTURE AND DENSITY OF STATES FOR $1T_d$ PHASES

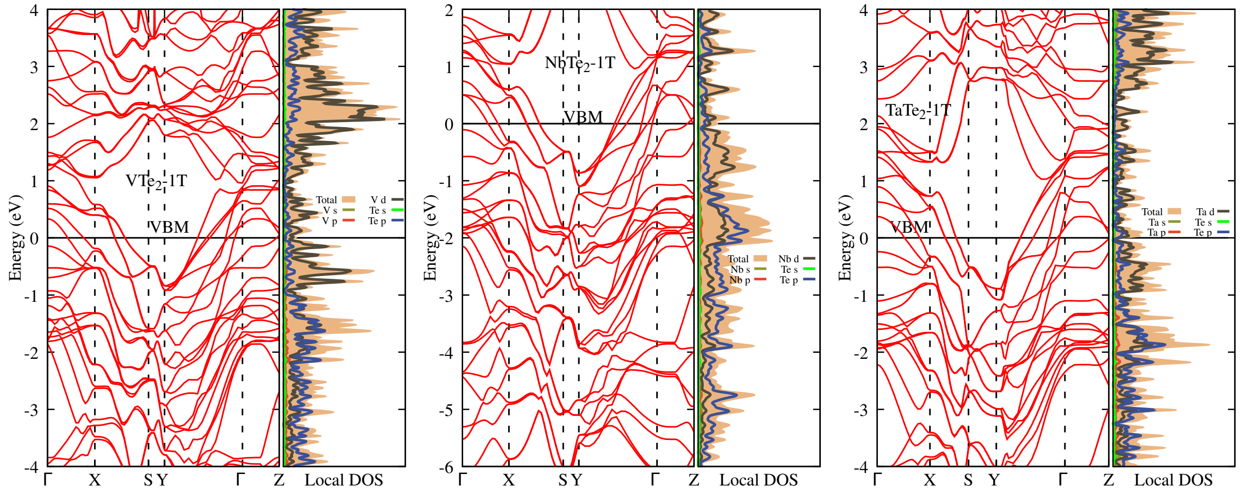


FIG. 13. 1Td: V, Nb, Ta

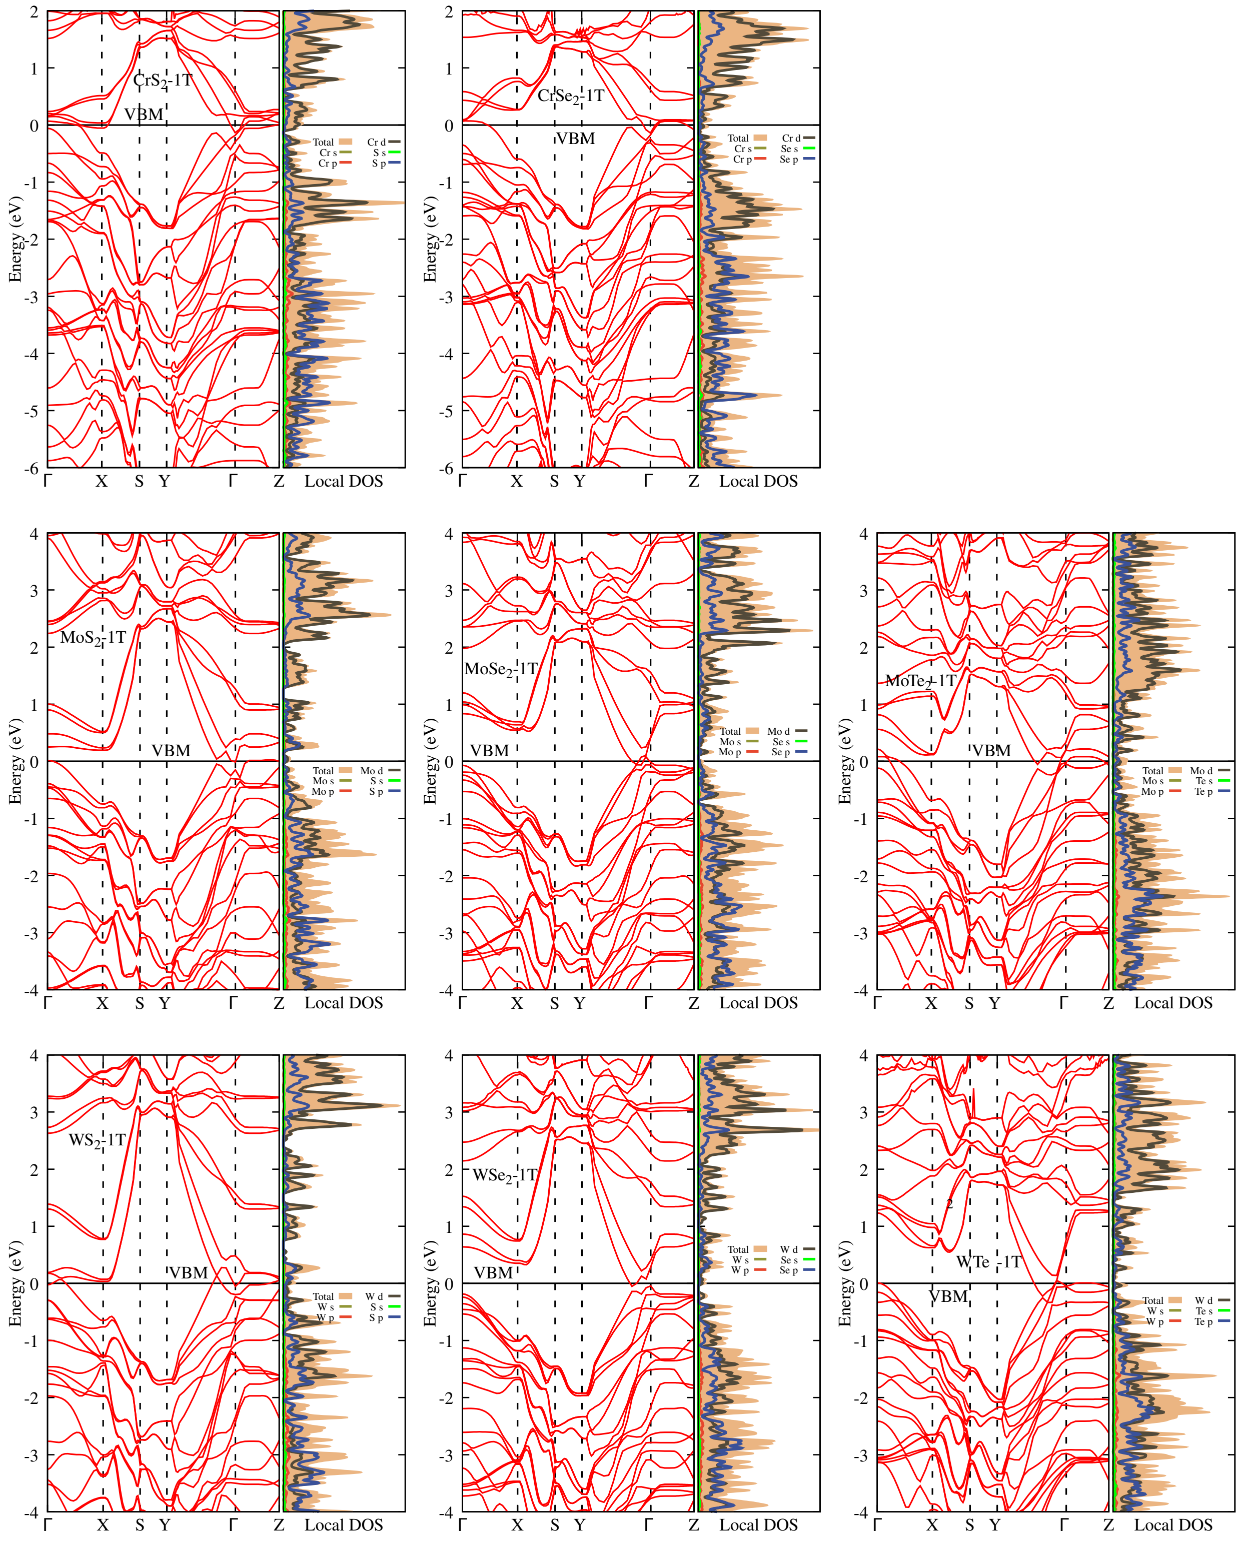


FIG. 14. 1Td: Cr, Mo, W
